# Supplementary material for: Berry curvature-induced local spin polarisation in gated graphene/WTe$_2$ heterostructures
Source: arXiv:2106.15509 source file (2021-06-29)
Supplement: Supplementary file 1 [file supplement.tex]

\clearpage
\onecolumngrid %change to single column document
\setcounter{figure}{0} %reset figure numbering
 %put "S" in front of figure number within supplement

\section{Supplementary Information}

\subsection{Raman spectroscopy}
\begin{figure}[h]
\includegraphics[scale=1]{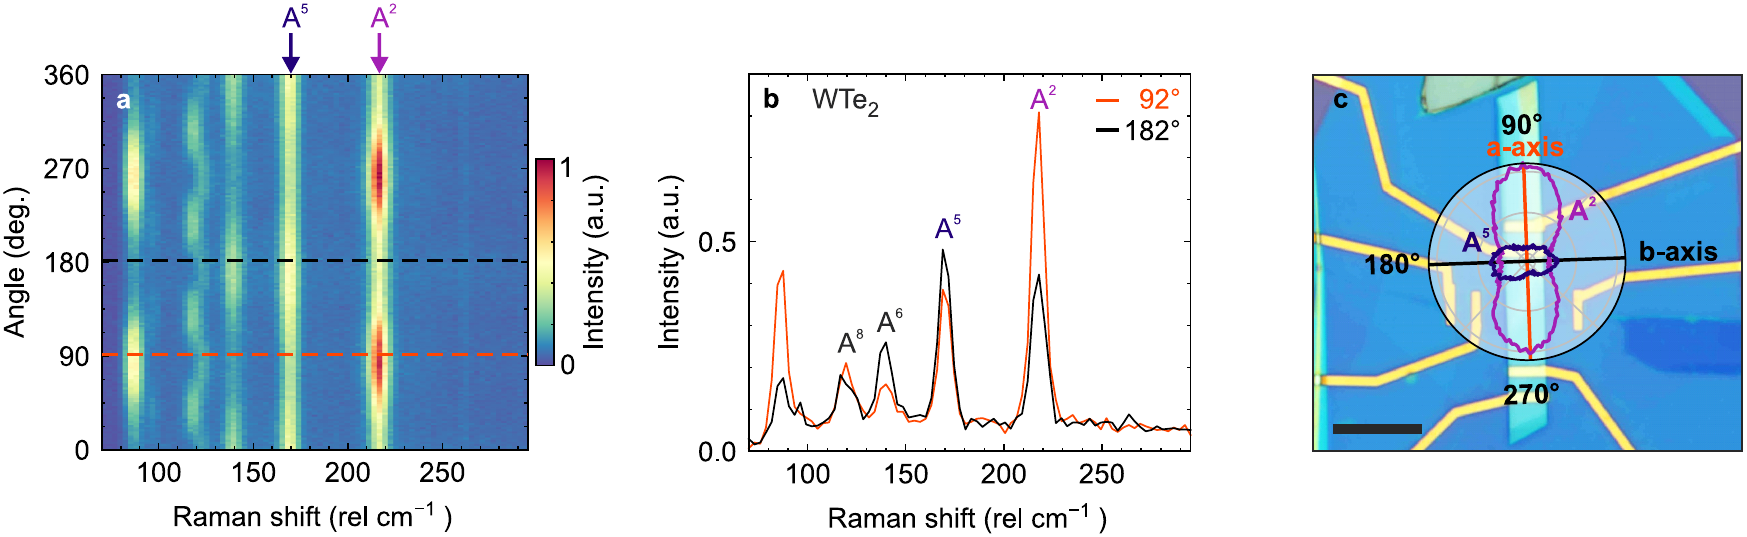}
\caption{\textbf{Raman scpectroscopy.} a) Polarisation-resolved Raman spectra of the \ch{WTe2} film for different linear excitation polarisations at room temperature. The linearly polarised laser excitation ($\lambda_\mathrm{exc}=\SI{532}{\nano\meter}$) is rotated with a half-waveplate. The signal is detected in co-polarisation configuration, i.e. excitation polariser and detection analyzer are parallel to each other. b) Raman spectra of the \ch{WTe2} film along its crystallographic $a$- (orange line) and $b$-axis (black line) colour coded in panels a) (dashed lines) and c) (vertical and horizontal lines), respectively. c) Optical image of the graphene/\ch{WTe2} cross-junction covered with hBN. A polarisation-dependent intensity polar plot of the $A^2$- (purple) and $A^5$-Raman modes (blue) is overlaid, confirming the crystallographic axis orientations. Scale bar is \SI{10}{\micro\meter}. }
\label{fig: SI_raman}
\end{figure}

% \subsection{Equivalent circuit model}

% \begin{figure}[h]
% \includegraphics[scale=1]{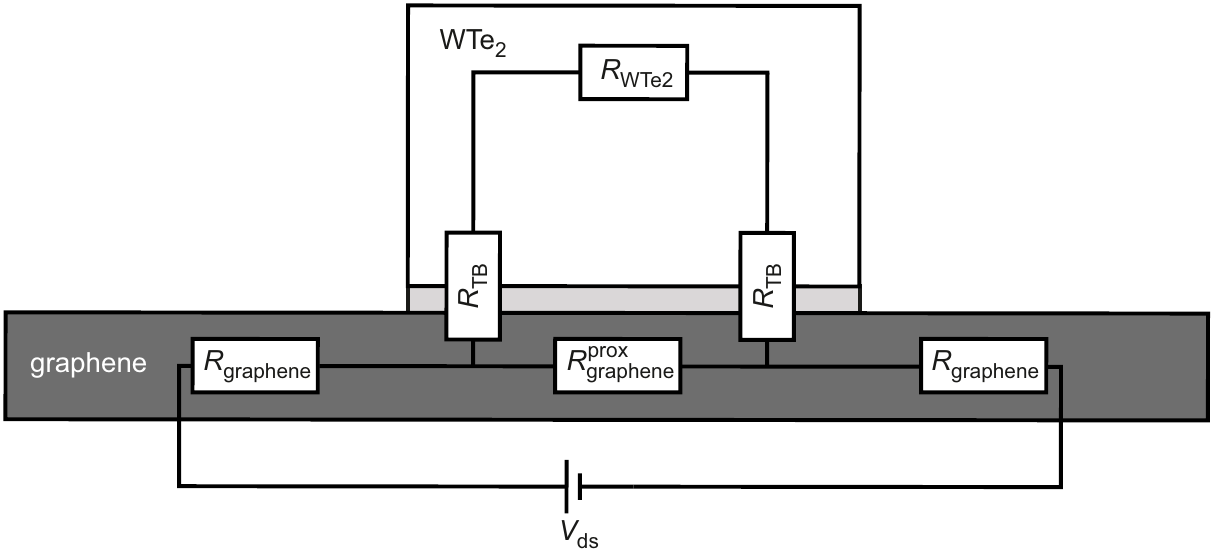}
% \caption{\textbf{Equivalent circuit diagram.} Resistance of the graphene leads $R_\text{graphene}$, tunnel barrier resistance $R_\text{TB}$, and resistance of the $\ch{WTe2}$ film $R_\text{WTe2}$.}
% \label{fig: SI_equivalent circuit}
% \end{figure}

\clearpage

\subsection{Mapping of local charge current}
With the aim of determining the spatial dependence of heat dissipation, i.e., the local current density and resistivity, we applied an alternating source-drain voltage with a frequency of $\omega=\SI{3.33} {\kilo\hertz}$ and monitored the KR on the frequency $2\omega$ by a lock-in measurement. Previous Kerr microscopy experiments on metals have shown that the Kerr signal $\theta_{K}^{2\omega}$ at modulation frequency $2\omega$ indeed captures the effect of Joule heating on the optical reflectivity of the sample \cite{stamm2017magneto}. Fig. \ref{fig: SI_dissipation} shows spatial maps of $\theta_{K}^{2\omega}$ around the WTe$_2$/graphene heterointerface, which were obtained in four different bias configurations. For source-drain bias applied across the junction, the maximum signal is always located along the direction of current flow, i.e., either to the right (Fig. \ref{fig: SI_dissipation}a) or the left (Fig. \ref{fig: SI_dissipation}b) towards the corresponding electrical contact on graphene.
It could be confirmed that the $2\omega$ signal scales approximately quadratic with the applied ac current amplitude as expected for Joule heating (see Supplementary Fig. \ref{fig: SI_kerr_sd_dependence}). Thus, we conclude that the signal demodulated at $2\omega$ indeed reflects the local dissipation and hence the local charge current density. On this basis, the signal maxima in Fig. \ref{fig: SI_dissipation}a and \ref{fig: SI_dissipation}b can be explained by a local vertical current flow between the two layers. In comparison, for in-plane biasing along the \ch{WTe2} channel, a much weaker signal occurs at the central interface, indicative of Joule heating within the less resistive WTe$_2$. Finally, when the bias is applied along the proximitized graphene, which is nominally in-plane, we detect an increased optical response from the edges indicating a significant out-of-plane component of the current (Fig. \ref{fig: SI_dissipation}d).
The two pronounced $2\omega$ Kerr signals for bias along graphene only (cf. Fig. \ref{fig: SI_dissipation}d) originate from a local out-of-plane current flow from graphene to WTe$_2$.

% reference  is [19] in text above

\begin{figure*}[hbt]
\includegraphics[scale=0.98]{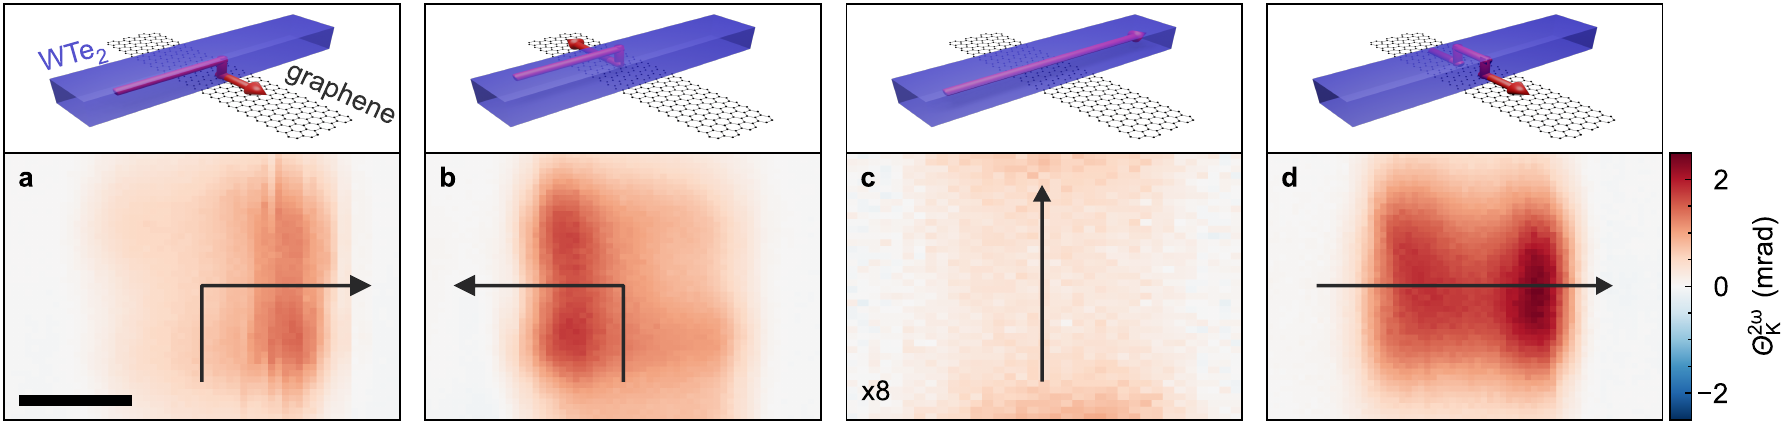}
\caption{\textbf{Mapping of local charge current.} Current-induced KR $\theta_{K}^{2\omega}$ (lower panel) for different bias configurations of the graphene/\ch{WTe2} junction (upper panel). (a) and (b) Bias applied between graphene and WTe$_2$. Bias applied along (c) WTe$_2$ and (d) graphene only. In (c), the colour scale was expanded by a factor of eight for better visibility. The arrows indicate the direction of the ac current as expected from the bias configuration and the location of the electrical ground. Scale bars are \SI{2}{\micro\meter}, $T_\text{bath} = \SI{4.2}{\kelvin}$, $V_\text{g} = \SI{0}{\volt}$, a) $V_\textbf{ds}$ = \SI{3}{\volt} b) $V_\textbf{ds}$ = \SI{3}{\volt}, c) $V_\textbf{ds}$ = \SI{4}{\volt}, d) $V_\textbf{ds}$ = \SI{1.5}{\volt}.} 
\label{fig: SI_dissipation}
\end{figure*}

\begin{figure}[hbt]
\includegraphics[scale=0.98]{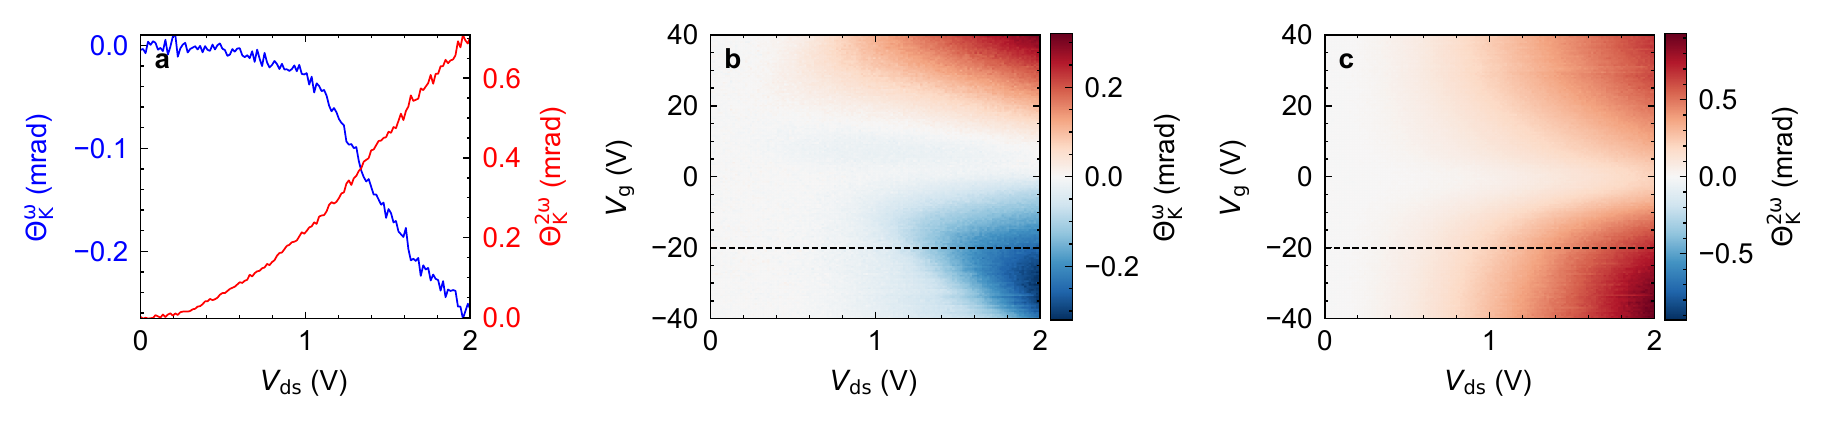}
\caption{\textbf{Bias- and gate-dependent KR microscopy.} a) First (blue line) and second harmonic (red line) KR signal as a function of ac bias along the graphene stripe, acquired on the junction edge at $V_\mathrm{g} = \SI{-20}{V}$. While the $2\omega$ KR scales approximately quadratic with the applied ac bias, the KR at the fundamental frequency $\omega$ exhibits a gate voltage-dependent onset. b)-c) First and second harmonic KR angle as a function of applied graphene ac bias and gate voltage. The dashed lines indicate the the traces depicted in panel a).}
\label{fig: SI_kerr_sd_dependence}
\end{figure}

\clearpage
\subsection{Data of additional samples}

\begin{figure}[h]
\includegraphics[scale=1]{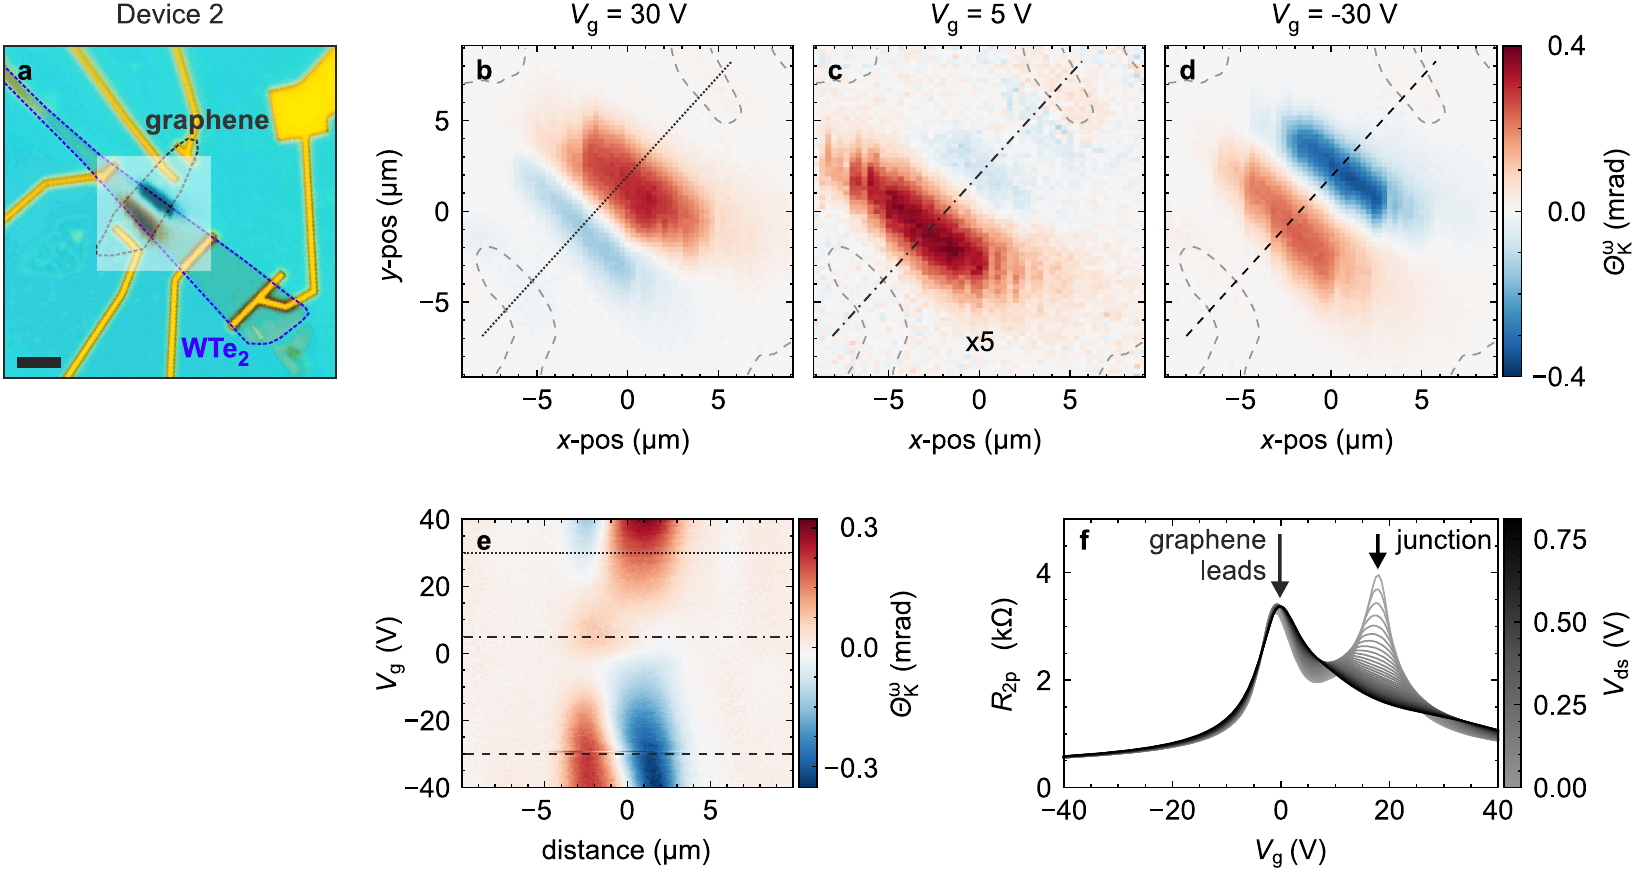}
\caption{\textbf{Extended data of a second device.} a) Optical microscopy image of a heterostructure comprised of graphene (black dashed line), \ch{WTe2} (blue dashed line), and hBN capping. Scale bar is \SI{5}{\micro\meter}. The overlay (shaded area) shows the current-induced KR signal at the junction using a colour code as in panel (d). b)-d) Spatially-resolved magneto-optic KR signal under ac current flow along the graphene stripe for (b) $V_\mathrm{g} = \SI{30}{V}$, (c) $V_\mathrm{g} = \SI{5}{V}$, (d) $V_\mathrm{g} = \SI{-30}{V}$. The Kerr angles are measured at the fundamental frequency $\omega$ of the alternating bias current. Grey dashed lines highlight the metal electrodes. The data in c) is scaled by a factor of 5 for clarity. $T_\mathrm{bath}=\SI{4.2}{K}$, $V_\mathrm{ds}=\SI{2}{V}$. e) Spatially-resolved KR $\theta_{K}^{\omega}$ across the graphene/\ch{WTe2} heterojunction as a function of applied gate voltage. Dotted, dash-dotted and dashed lines correspond to profiles indicated in panels b), c), and d), respectively. f) Transfer curves of the graphene stripe within the device in panel (a), measured in 2-probe configuration at $T_\mathrm{bath} = \SI{4.2}{K}$ using an ac voltage that increases stepwise up to \SI{0.8}{V}.}
\label{fig: SI_device2}
\end{figure}

\begin{figure}[h]
\includegraphics[scale=1]{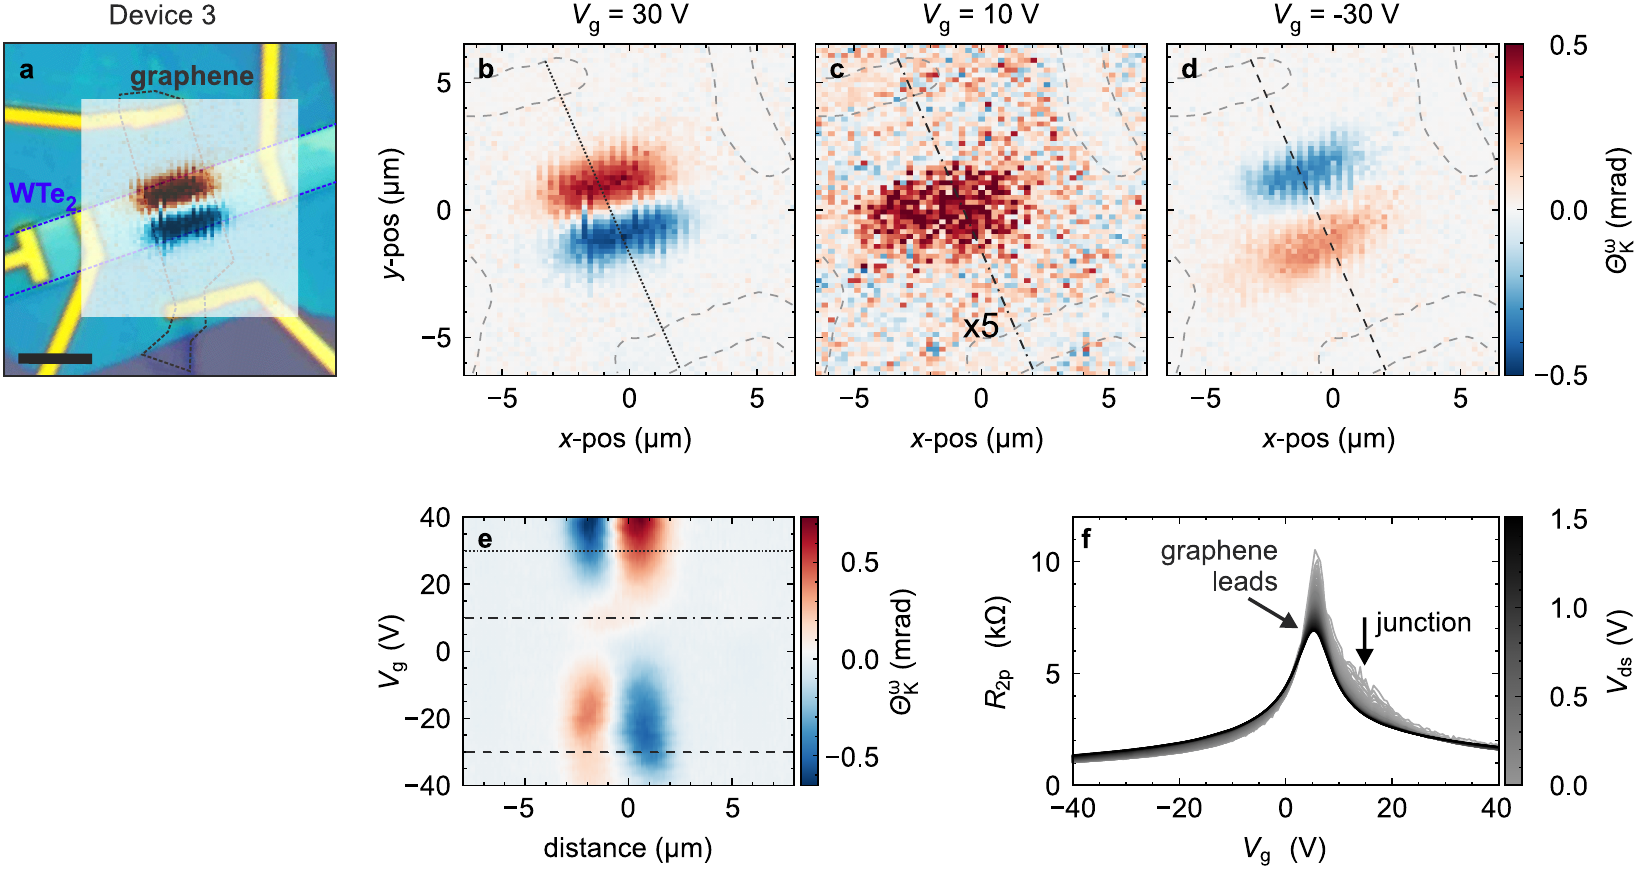}
\caption{\textbf{Extended data of a third device.} a) Optical microscopy image of a heterostructure comprised of graphene (black dashed line), \ch{WTe2} (blue dashed line), and hBN capping. Scale bar is \SI{5}{\micro\meter}. The overlay (shaded area) shows the current-induced KR signal at the junction using a colour code as in panel (d). b)-d) Spatially-resolved magneto-optic KR signal under ac current flow along the graphene stripe for (b) $V_\mathrm{g} = \SI{30}{V}$, (c) $V_\mathrm{g} = \SI{5}{V}$, (d) $V_\mathrm{g} = \SI{-30}{V}$. The Kerr angles are measured at the fundamental frequency $\omega$ of the alternating bias current. Grey dashed lines highlight the metal electrodes. The data in c) is scaled by a factor of 5 for clarity. $T_\mathrm{bath}=\SI{4.2}{K}$, $V_\mathrm{ds}=\SI{3}{V}$. e) Spatially-resolved KR $\theta_{K}^{\omega}$ across the graphene/\ch{WTe2} heterojunction as a function of applied gate voltage. Dotted, dash-dotted and dashed lines correspond to profiles indicated in panels b), c), and d), respectively. f) Transfer curves of the graphene stripe within the device in panel (a), measured in 2-probe configuration at $T_\mathrm{bath} = \SI{4.2}{K}$ using an ac voltage that increases stepwise up to \SI{1.5}{V}.}
\label{fig: SI_device3}
\end{figure}

\clearpage
\subsection{Experimental setup}

\begin{figure}[h]
\includegraphics[scale=0.98]{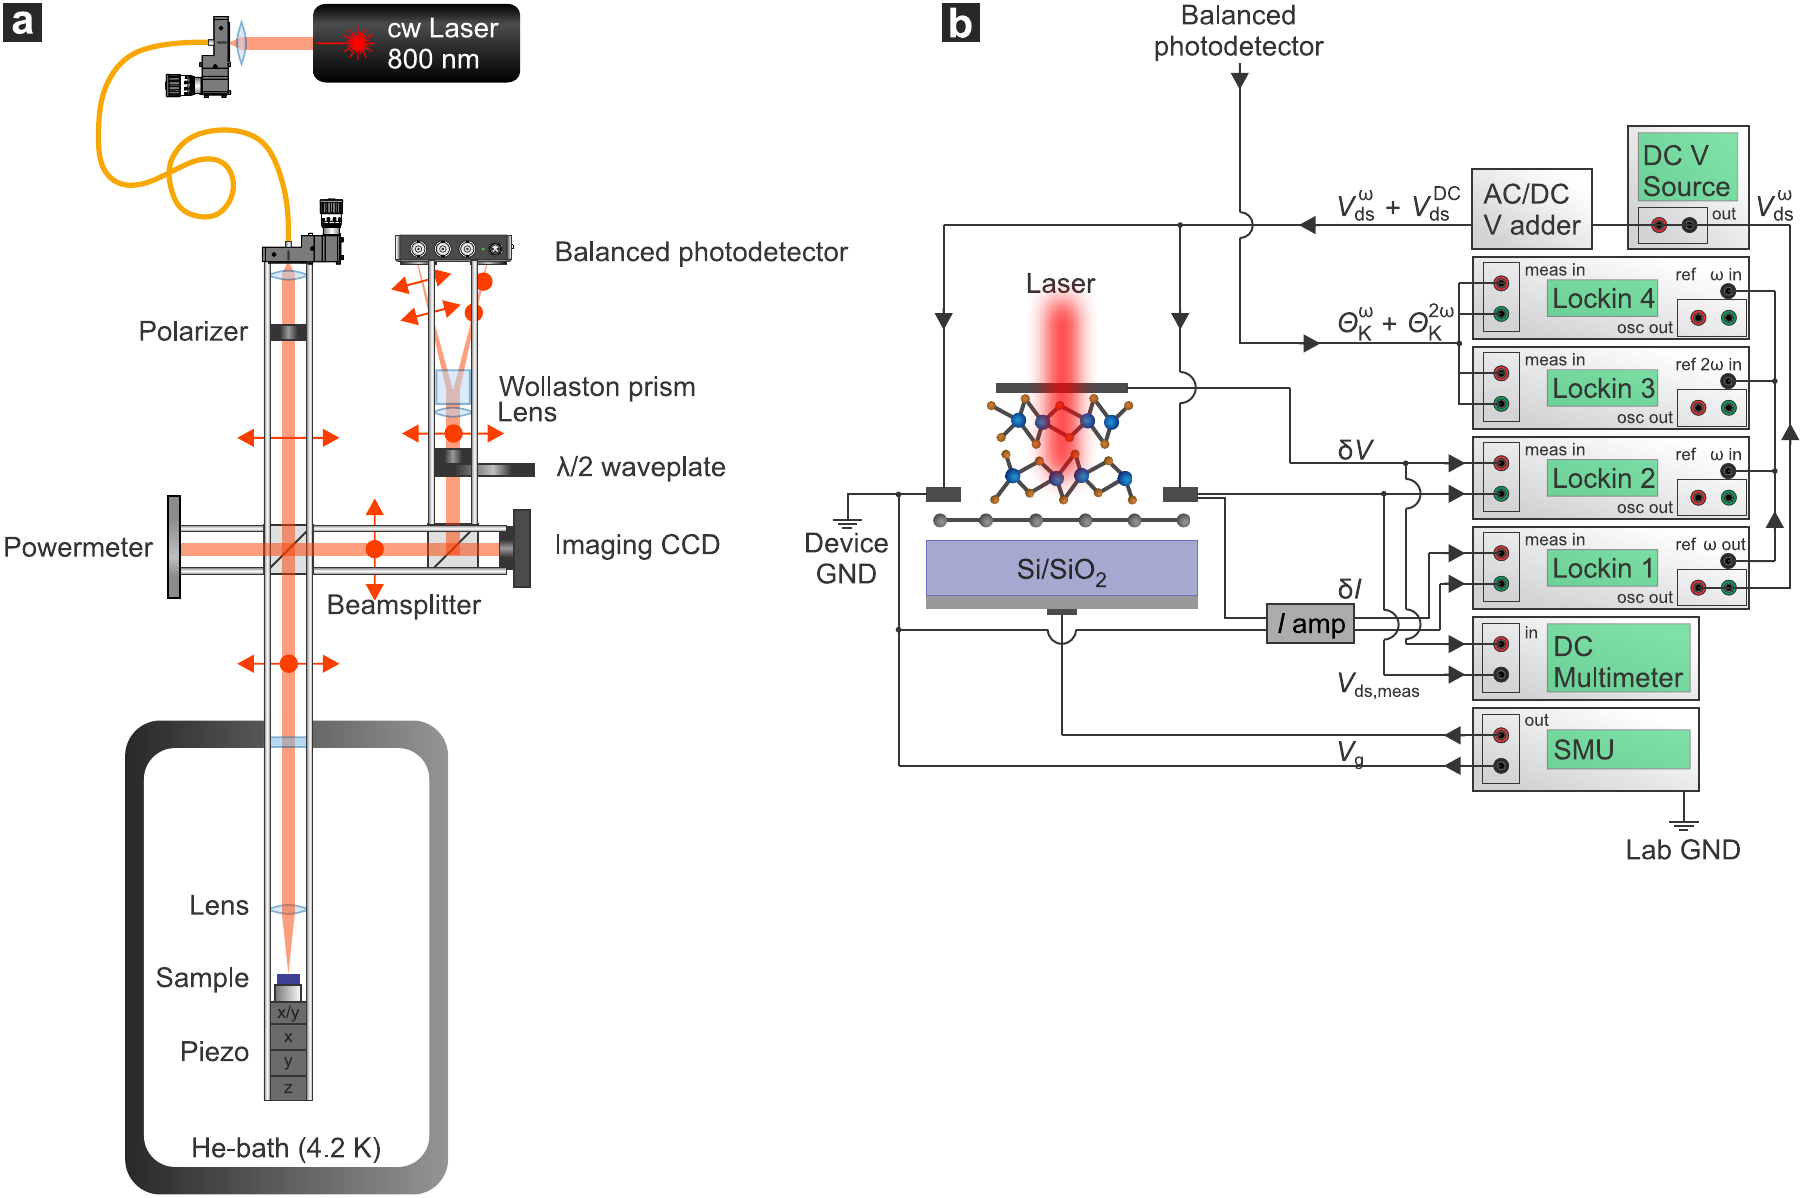}
\caption{\textbf{Opto-electronic setup.} a) Schematic of the used confocal dip-stick microscope with a sample bath-temperature of \SI{4.2}{K}. A linearly polarised cw-laser at $\lambda_\mathrm{laser}=\SI{800}{nm}$ is focused onto the sample with a diffraction-limited spot-size of $\sim \SI{800}{nm}$. The reflected beam is guided through a 50:50 beamsplitter, a half-wave plate, a Wollaston prism, and focused onto an amplified balanced photodetector. For spatially-resolved photocurrent measurements, the laser is chopped at a frequency of $\SI{3.33}{kHz}$. Spatially-resolved scanning is performed by moving the sample with a $xy$-piezo scanner mounted on top of a $xyz$-piezo stepper. b) Schematic electronic setup for the readout of current-induced KR, tunnelling, and photocurrent measurements. A small ac bias voltage $V_\mathrm{ds}^{\omega}$ (\SI{1}{mV} at \SI{77}{Hz}) is added to a dc bias voltage $V_\mathrm{ds}^\mathrm{DC}$ which are applied between source and drain contacts (e.g. across graphene or across the graphene/\ch{WTe2} junction). The resulting change in current flow is pre-amplified and monitored with a lock-in amplifier at the fundamental frequency $\omega$. Concurrently, the ac and dc voltage drop across the \ch{WTe2} (or the junction) is measured using a second lockin amplifier and a dc multimeter. As a function of applied gate voltage $V_\mathrm{g}$ (source/measure unit SMU) and bias voltage $V_\mathrm{ds}^{\omega} + V_\mathrm{ds}^\mathrm{DC}$, the KR signal is measured by decomposing the output of the balanced phtotodetector into its first two harmonic components $\theta_{K}^{\omega}$ and $\theta_{K}^{2\omega}$ using two additional lock-in amplifiers.}
\label{fig: SI_experimental_setup}
\end{figure}

\clearpage

\subsection{Theory - Derivation of Kerr response}

In this section, we present details on the Kerr response and topological extension of Fick theory and its solution for the problem of the WTe$_2$ slab on the graphene strip. 

\subsection*{Kerr response}

We remind the reader that the Kerr angle is given by 
\begin{equation}
    \theta_K = - \text{Re} \frac{\sigma_H^{\rm 2D}}{\sigma^{\rm 2D}}.
\end{equation}
This equation directly follows from classical electrodynamics in the limit when the gyrotropic material is thin as compared to the wavelength of light. In this limit, $\sigma^{2D} (x,y) = \int_0^h dz \sigma (x,y,z)$ is sheet conductance (which for simplicity of notation is taken isotropic, here). The 2D Hall conductance is defined analogously (see also main text).

\subsection*{Topological Fick theory}

The Boltzmann equation describing a generic topological material is given by

\begin{equation}
    \dot f + \dot{\mathbf r} \partial_{\mathbf r} f + \dot{\mathbf p}\partial_{\mathbf p} f = St[f],
\end{equation}
where $St[f]$ denotes the collision integral which we treat in the relaxation time approximation, $\dot{\mathbf p}$ is given by the external force (Newton's law) and $\dot{\mathbf r} = \mathbf v + \boldsymbol \Omega \times \dot{\mathbf p}$ ($\mathbf v$ is the derivative of the dispersion relation $\epsilon(\mathbf p)$ and $\boldsymbol \Omega = \boldsymbol \Omega (\mathbf p)$ is the Berry curvature). We define density, current density and Berry curvature density as $n = \int (dp) f, \mathbf j = \int (dp) \mathbf v f, and  \boldsymbol \omega = \int (dp) \boldsymbol{\Omega} f$, respectively, where $(dp) = d^d p/(2\pi)^d$ is the measure of momentum integrals. 

To derive the topological Fick diffusion theory, we assume fast equilibration of the distribution function $f(\mathbf p, \mathbf r, t)$, and replace, $\int (dp) v_i v_j \partial_{x_j} f$ with $\partial_{x_j} n D^{ij}/\tau$, where $D^{ij} = \langle v^i v^j \rangle_{\rm FS} \tau$ and $\langle \dots \rangle_{\rm FS}$ is the average over the Fermi surface. Similar replacements occur in other quantities. Then, Fick's first law (i.e. the diffusive relationship between current and density) follows from multiplying the Boltzmann equation with $v_i$ and subsequent integration $\int(dp)$ of the entire equation (assuming that the current dynamics is slow with respect to $\tau$). The second law is the continuity equation obtained by just integrating the Boltzmann equation. The topological extension is obtained by multiplying the equation by $\boldsymbol \Omega$ before integration. This concludes the derivation of Fick diffusion theory.

Next, we comment on the source term for the coupled heterostructure. Using $w_{t,\mathbf r, \mathbf p},$ and $g_{t,\mathbf r, \mathbf p}$ to denote the time $t$, position $\mathbf r$ and momentum $\mathbf p$ dependent distribution function in WTe$_2$ and graphene, respectively, we consider the following corrections to the collision integral
\begin{subequations}
\begin{eqnarray}
\delta St_{w}[w,g] &=& -\int \frac{d^2 p'}{(2\pi)^2} \omega_{\mathbf p, \mathbf p'
 } [w_{t,\mathbf r, \mathbf p} - g_{t,\mathbf r, \mathbf p'}] c \delta(z)\chi(x,y),\\
  \delta St_{g}[w,g] &=& -\int \frac{d^3 p'}{(2\pi)^3} \omega_{\mathbf p', \mathbf p
 }c [g_{t,\mathbf r, \mathbf p} - w_{t,\mathbf r, \mathbf p'}]_{z = 0}\chi(x,y).
 \end{eqnarray}\label{eq:exchange}
 \end{subequations}
It describes the particle exchange at the interface (in an idealized situation, $\chi(x,y) = 1$ where graphene and WTe$_2$ overlap and zero otherwise). This explains the appearance of the delta function $\delta(z)$ (the constant $c$ is the size of the unit cell in WTe$_2$ in z-direction). For simplicity, we will model $\omega_{\mathbf p, \mathbf p'} = \omega_0 \delta_{\mathbf p_\Vert, \mathbf p'} + \omega_1$ (accounting for completely momentum conserving and completely momentum scrambling contributions, respectively). Note that all perpendicular plane waves in WTe$_2$ with arbitrary $p_z$ couple to the graphene, as they all have some weight on the $z = 0$ surface. 
 
With these assumptions, the collision integral leads to  the following modifications of the continuity equation and the Fick's laws:  

(i) The continuity equation (essentially Fick's second law) obtains an addition which is given by particle density exchange between graphene and WTe$_2$. This term stems from both $\omega_0,\omega_1$ and is responsible for the charge transfer in equilibrium. As we are interested in the non-equilibrium transport setting, we perturb about this induced equilibrium state. We effectively account for it by imposing different equilibrium density underneath the junction and in the graphene leads, and therefore will not discuss the effect of $\omega_1$, explicitly.
 
(ii) The First Fick's law, obtained by first multiplying the Boltzmann equation with $v_i$ and then integration, contains additional terms of current exchange at the interface,
 \begin{eqnarray}
 \frac{D^{ij}_w}{\tau_w} \partial_j n_w &=& - \frac{j_w^i}{\tau_w} + \alpha_w \frac{\bar D^{ij}_w \partial_j n_g}{\tau_w} \delta(z), \\
 \frac{D^{ij}_g}{\tau_g} \partial_j n_g &=& - \frac{j_g^i}{\tau_g} + \alpha_g \frac{\bar D^{ij}_g \partial_j n_w}{\tau_g} \vert_{z = 0}.
 \end{eqnarray}
Here, $\alpha_{w,g}$ are constants proportional to $\omega_0$. The constants $\bar D^{ij}_w = \langle v^i_w v_g^j \rangle_{\rm ( FS \; of \; graphene)} \tau_w$, $\bar D^{ij}_g = \langle v^i_g v_w^j \rangle_{\rm (FS \; of \; WTe_2)} \tau_w$ are generated from Eqs.~\eqref{eq:exchange} using the assumption of fast equilibration. Note that $\bar D^{ij}$ is opposite for electron or hole carriers in graphene. This is the origin of the ambipolar nature of the effect discussed in the main text. 

In the following, we simplify these equations, by setting $D^{ij}_w = D \delta^{ij}$, $D^{ij}_g = D_g \delta^{ij}$, $\alpha_w \bar D^{ij}_w = \bar D_w \delta^{ij}$, $\alpha_g \bar D^{ij}_g =ca \bar D_g \delta^{ij}$ (where $c$ is a UV length scale and $D_g$ the diffusion constant in graphene). We also fix $\bar D_w >0$ and absorb the sign of $\bar D_w$ into the density: Ultimately, the source term for the current becomes $\pm \bar D_w \partial_{\mathbf x} n_g$ (with the sign being positive/negative in conduction/valence band) - this is the origin of the coupling to the imbalance current discussed in the main text (there, the subscript ``$_w$'' is omitted from $\bar D_w$).

Finally, we briefly consider the correction to the topological extension
\begin{equation} \label{eq:omegacorr}
    D_{ji}^{(\Omega)} \partial_j n_w = -\frac{\varpi_i}{\tau_w} + \bar \alpha \frac{\bar D_{ji}^{(\Omega)} \partial_j n_g}{\tau_w} \delta(z).
\end{equation} 
The symmetry properties of both $ D_{ji}^{(\Omega)}$ and $ \bar D_{ji}^{(\Omega)}$ are the same as those of $\lambda_{ji}$ discussed in the main text - the only non-zero contribution is $i = j = z$, but there is no current in graphene in $z$-direction. Hence, the correction in Eq.~\eqref{eq:omegacorr} vanishes.

\subsection*{Imbalance decay}

Before going into the details of the diffusion equations for the heterostructure, we briefly consider imbalance relaxation in pure graphene. In this supplement, we use the notation for currents and densities $j_w = - D\nabla n_w, j_I = - D_g \nabla n_I$, and $j_q = - D_g \nabla q$, where $n_w$ is the density in WTe$_2$. We use the notation of imbalance density $n_I = n_e + n_h>0$ and charge density $q = n_e - n_h$, where $n_e$ and $n_h$ are electron and hole density, respectively. We stress that the electron and hole density are space-dependent even in equilibrium (due to local charge transfer under the WTe$_2$ strip). However, per definition the static solution is current free and the corrections to the equilibrium solution vanish. Details of this notation follow in the next section.

Imbalance relaxation occurs through decays $e^{-} \rightarrow e^{-} + e^{-}  +h^{+}$, and is therefore a non-linear function of densities. Moreover, at finite doping, the minority carrier density vanishes in equilibrium and zero temperature: In this case $n_I = \vert q \vert$, while in general (e.g. not at equilibrium) $n_I\geq \vert q \vert$. All of these aspects are encoded in the following addition to the continuity equation of the imbalance density $n_I$ 
\begin{equation}
\dot n_I - D_g \nabla^2 n_I = - \frac{n_I^2 - q^2}{2q_0^2} \frac{n_I}{\tau_{\rm rec}}.
\end{equation}
Here, $\tau_{\rm rec}$ is the recombination rate, which is typically macroscopically large. The charge $q_0$ is the externally imposed charge density, which is modelled by a piecewise constant function. Then, we linearize these equations around the equilibrium value. The coupled equations of interest between graphene and WTe$_2$ are thus
\begin{eqnarray}
- D \nabla^2 n_w &=& - \alpha\partial_x [\bar D_w \partial_x n_I ] \delta(z), \label{eq:DiffWTe2}\\
%- D_g \partial_x^2 q &=&0, \\
 - D_g \partial_x^2 n_I &=& - \frac{n_I - \vert q \vert}{\tau_{\rm rec}}-\partial_x [a\bar D_g \partial_x n_w]_{z = 0},
\end{eqnarray}
supplemented with charge conservation, which implies $\dot{n}_w + \dot q + \nabla(j_w + j_q) = 0$. For simplicity, we consider time- and $y$-independent solutions which is the reason for dropping time and $\partial_y$ gradients. %\imEJK{might need to be changed into $y \rightarrow x \rightarrow - y$ everywhere, depending on orientation of the sample.} 
We further apply a transport current, such that charge conservation implies $j_q + \int_0^h dz j_{W,x} = j_0 = \text{const.}$.

We will assume that the hybridization $\bar D_w = \bar D_g = 0$ at the boundary $x = \pm l/2$, and that it sets on in a smooth rapid fashion beyond the boundary (i.e. it is spatially dependent). At the same time, diffusion constants are assumed spatially independent.

In these equations we have focussed on the effect of momentum transfer between graphene and WTe$_2$, i.e. a current in WTe$_2$ imposes an imbalance current in graphene and vice versa. We exploit that a non-zero momentum transfer can always be expected at the interface and it is the minimal ingredient for the Kerr response. Charge transfer, which might also be present but does not affect current injection and the Kerr response, is neglected here.

\subsection*{Green's function in WTe$_2$}
Let $G(x,x';z,z')$ be the Green's function, i.e. $ \nabla^2 G(x,x';z,z') = \delta(x- x') \delta(z-z')$ of the Laplacian inside the WTe$_2$ sample, $(x,z)\in(-l/2,l/2)\times(0,h)$ with von-Neumann boudnary condition $\mathbf j \cdot \hat {\mathbf n} = 0$. (Note that this does not impede tunnelling into or out of the sample.) 

The Green's function of the 2D Laplacian is $G_0(x,z) = \ln(x^2 +z^2)/(4\pi)$. The no outflux boundary conditions can be imposed by an infinite sequence of (mirror) charges located at $(x_n,z_m) = (2n l + x', 2m h + z')$, $(x_n,z_m) = ((2n +1)l - x', 2m h + z')$, $(x_n,z_m) = ((2n +1)l - x', 2m h + z')$, $(x_n,z_m) = (2n l x', 2m h - z')$ and $(x_n,z_m) = ((2n +1)l - x', 2m h - z')$.

Deep inside the strip of height $h \ll l$, the Green's function is dominated by charges at $x = x'$ in which case 
\begin{equation}
G(x,x'; z,z') = \frac{1}{4\pi}\left \lbrace \ln \left [\cosh(\frac{\pi(x - x')}{h})-\cos(\frac{\pi(z - z')}{h})] +  \ln [\cosh(\frac{\pi(x - x')}{h})-\cos(\frac{\pi(z + z')}{h})\right]\right \rbrace.
\end{equation}
Assuming both $x$ and $x'$ at distances larger than $h$ from the boundary, we obtain
%in this regime, which assumes both $x$ and $x'$ at distance larger than $h$ from the boundary,
\begin{subequations}
\begin{eqnarray}
\int_0^h dz \partial_x G(x,x'; z,0) &=& \frac{\text{sign}(x-x')}{2},  \\
\int_0^h dz \partial_z G(x,x'; z,0) &=& \frac{1}{2\pi}\ln\left ( \frac{\cosh(\pi (x-x')/h)+1}{\cosh(\pi (x-x')/h)-1}\right).
\end{eqnarray}
For trial functions, which are smooth on the scale $h$ one may further approximate
\begin{eqnarray}
\partial_x G(x,x'; z,0) &\simeq & \frac{\text{sign}(x-x')}{2h},  \\
\int_0^h dz \partial_z G(x,x'; z,0) &\simeq&  \frac{h}{\pi} \delta(x-x'). 
\end{eqnarray}
\label{eq:ApproxG}
\end{subequations}

%We also remark that $(\partial_x, \partial_z) G_0(x,z) = (\partial_z, -\partial_x) \psi_0(x,z)$, where $\psi_0(x,z) = \arctan(z/x)/(2\pi)$ is the phase winding about the origin. Using an analogous notation as for the Green's function, we denote $\psi(x,x';z,z')$ the sum over arcustangens functions centered about mirror charges.

\subsection*{Solution of diffusion equation in WTe$_2$}
Using the Green's function, the solution of the diffusion equation, Eq.~\eqref{eq:DiffWTe2}, is
\begin{subequations}
\begin{equation}
n_w(x,z) = \int_{-l/2}^{l/2} dx'  G(x,x';z,0) \partial_{x'}[\bar D_w \partial_{x'}n_I]/D,
\end{equation}
which implies in terms of currents
\begin{eqnarray}
\mathbf j_{w} &=& \int_{-l/2}^{l/2} dx' \nabla G(x,x';z,0) \partial_{x'}\left [\frac{\bar D_w}{D_g} j_I(x') \right].
\end{eqnarray}
We use this, as we determine the total currents in the sample,
\begin{eqnarray}
j_x^{\rm tot} \equiv  \int_0^h dz j_{w,x} &=& \int_{-l/2}^{l/2} dx' \int_0^h dz \partial_x G(x,x';z,0) \partial_{x'} \left [\frac{\bar D_w}{D_g} j_I(x') \right] \notag\\
&=&\int_{-l/2}^{x} \frac{dx'}{2}\partial_{x'} \left [\frac{\bar D_w}{D_g} j_I(x')\right ] - \int_{x}^{l/2} \frac{dx'}{2}\partial_{x'} \left [\frac{\bar D_w}{D_g} j_I(x') \right ]\notag \\
&=& \frac{\bar D_w}{D_g} j_I(x),\\
j_z^{\rm tot} \equiv  \int_0^h dz j_{w,x} &=& \int_{-l/2}^{l/2} dx' \int_0^h dz \partial_z G(x,x';z,0) \partial_{x'} \left [\frac{\bar D_w}{D_g} j_I(x') \right]\notag\\
&=&\int_{-l/2}^{l/2} dx'[ G(x,x';h,0)- G(x,x';0,0)] \partial_{x'} \left [\frac{\bar D_w}{D_g} j_I(x') \right] \notag \\
&\simeq & \frac{h}{D_g\pi} \partial_x [\bar D_w j_I]. 
\end{eqnarray}
Here, we made use of Eqs.~\eqref{eq:ApproxG}, which are valid at positions $x,x'$ which are distant $h$ or larger from the boundary. We thus found that the Kerr angle is directly proportional to $\partial_x j_I(x)$. A smooth $\bar D_w j_I(x)$ allows to write 
\begin{equation}
j_x(x,z) \simeq \frac{\bar D_w}{h D_g} j_I(x).
\end{equation}
\label{eq:jzTot}
\end{subequations}

Note that $\bar D_w j_I$ varies on the scale of the imbalance relaxation length, which is macroscopic and substantially exceeds $h$. Therefore, $\vert j_z \vert \ll  \vert j_x \vert$.

It is furthermore obvious, that only those current configurations with $\int dx \partial_x{ \frac{\bar D_w}{h D_g} j_I(x)} = 0$ can satisfy the requirement of no current outflux. Since the same amount of current flows into WTe$_2$ and out of WTe$_2$ near either edge, this naturally explains the dominant antisymmetric spatial dependence of $\theta_K(x)$. At the same time, the contribution to $\theta_K(x)$ with a non-zero spatial average must stem from a different, weaker effect.

\subsection*{Solution of the diffusion equation in graphene}

We use Eq.~\eqref{eq:jzTot} in the diffusion equation for graphene, which becomes
\begin{equation}
- D_{\rm eff} \nabla^2 n_I = - (n_I - \vert q \vert)/\tau_{\rm rec},
\end{equation}
where $D_{\rm eff} = D_g + \frac{a \bar D_g \bar D_w}{h D_g D}$. The solution to this equation leads to
\begin{eqnarray}
j_I  &=& \text{sign}(q) j_{q,0} + \bar j_I \frac{\cosh(x/l_{\rm rec})}{\cosh(l/2l_{\rm rec})} + \delta j_I \frac{\sinh(x/l_{\rm rec})}{\sinh(l/2l_{\rm rec})}, \label{eq:ji}
\end{eqnarray}
where $l_{\rm rec} = \sqrt{D_{\rm eff} \tau_{\rm rec}}$ is the mean recombination path and we express the two boundary conditions by $\bar j_I, \delta j_I$, where $\text{sign}(q_0)  j_{q,0} + \bar j_I \pm \delta j_I/2$ are the imbalance currents at $x = \pm l/2$ (here, $q_0$ is the equilibrium density underneath the junction).

\subsection*{Boundary conditions}

We now model the boundary conditions on $j_I$ with the following two main requirements
\begin{itemize}
\item The boundary current is odd in the externally applied current $j_{q,0}$,
\item and odd under particle hole transformation.
\end{itemize}
The last point derives from the requirement that deep in the bands, $j_I \propto \text{sign}(q) j_q$ and is equivalent to inverting energy about the Dirac node, i.e. $j_I \propto \text{sign}(\mu - E_{\rm Dirac}) j_{q}$ near equilibrium. This motivates the following Ansatz
\begin{subequations}
\begin{eqnarray}
 \bar j_I &=& \mathcal C\underbrace{\frac{1}{\pi} \left \lbrace \arctan([\mu-E_{\rm out}] \tau)  + \arctan([\mu-E_{\rm in}] \tau)\right \rbrace}_{f(\mu)}j_{q,0} , \\
  \delta j_I &=& \mathcal C\frac{\delta \mu}{2\pi} \frac{\partial}{\partial \mu} \left \lbrace \arctan([\mu-E_{\rm out}] \tau)  + \arctan([\mu-E_{\rm in}] \tau)\right \rbrace j_{q,0},
\end{eqnarray} 
\label{eq:Boundary}
\end{subequations}
where $E_{\rm out}, E_{\rm in}$ are the energy of the Dirac point outside and inside the junction, respectively. Note that $\bar j_I, \delta j_I$ are boundary conditions on the correction to the imbalance density $n_I - \vert q \vert = n + p - \vert n - p \vert$, which is nothing but the minority charge. Therefore, the constant $\mathcal C$ becomes nonezero only when the bias voltage exceed the distance to the Dirac node, as observed in experiment.

\subsection*{Kerr response}

The current-induced Hall response in WTe$_2$ is $\sigma_H = \tau_w D^{(\Omega)}_{zz} \int_0^h dz \partial_z n_w = - \tau_w D^{(\Omega)}_{zz} j_z^{\rm tot}/D $. The Kerr angle is thus	
\begin{equation} \label{eq:thetaKerrFinal}
\theta_K = \frac{\sigma_H}{\sigma_w^{\rm tot} + \sigma_g} \simeq \frac{-  h \tau_w D^{(\Omega)}_{zz} \partial_x [\bar D_wj_I]/(D_g D)}{h D \nu_w}.%\\\frac{\tau_w D_{zz}^{(\Omega)}}{D_g D^2 \nu_{w}} \partial_x[ \bar D_w j_I].
\end{equation}

We can estimate the strength as follows
\begin{eqnarray}
\theta_K &\sim& \frac{\bar D_w D_{zz}^\Omega \tau_\omega}{D_g D^2 \nu_W l_{\rm rec}} j_{q,0} \sim \frac{\Omega}{v_F^2 \nu_w} \frac{1}{\ell l_{\rm rec.}} j_{q,0} \sim \frac{1}{p_F^2 \ell l_{\rm rec}} \frac{1}{W p_F} \frac{I}{e E_F}.
\end{eqnarray}

Here, some constants of order unity have been dropped: the transparency of the graphene and WTe$_2$ junction and $\mathcal C$  (for the contribution due to $j_I$).
For $I \sim \SI{1}{mA}$, $E_F \sim \SI{100}{meV}$ (in WTe$_2$), the factor is $I/(e E_F) \sim 40$. Choosing realistic numbers for the other parameters $p_F \ell \sim 10$, $W p_F \sim 100$, $l_{\rm rec} p_F \sim 100$ lead to $\theta_K \sim \text{mrad}$ at $I = \SI{1}{mA}$.

\subsection*{Fit to experiment}

It is important to keep in mind that the local $j_z^{\rm tot}(x)$ in WTe$_2$ can only account for the Kerr response which average to zero over the entire sample. Differently stated: The condition that current can only leave WTe$_2$ at the interface with graphene does not allow for a non-zero $\int dx j_z^{\rm tot}(x)$. Therefore, we here subtract the mean $\bar \theta_K(V_\mathrm{g}) = \int dx \theta_K(x,V_\mathrm{g})$ from the measured Kerr response at each value of gate voltage, see Fig.~\ref{fig:KerrFit}

Motivated by the theoretical relationship, Eqs.~\eqref{eq:jzTot},\eqref{eq:ji},\eqref{eq:thetaKerrFinal}, we expand in small $l \ll l_{\rm rec}$, and fit the data to the following simplified functional form
\begin{equation}\label{eq:thetaFit}
\theta_K = \frac{\partial \left[g(x,l_{\rm hyb})^2 \left(\left \vert V_\mathrm{g} \right \vert \left(A-B x^2\right) f(V_\mathrm{g})+C x\right)\right ])}{\partial x},
\end{equation}
where we set the position of the Dirac node outside (underneath) the junction $E_{\rm out} = 0$ ($E_{\rm in} = 24 V$, based on the position of the second maximum in the two-point resistance). Note the additional factor of $V_\mathrm{g}$ which also derives from the relationship between current and voltage in the regime of sufficiently large bias. 

The fit parameters are obtained using the Levenberg-Marquardt algorithm implemented in \textit{Mathematica} and reported in Tab.~\ref{tab:TabValues}. 
The comparison to the experimental data, Fig.~\ref{fig:KerrFit} highlights that major aspects are reproduced, particularly the ambipolar nature of the effect and the sign change as a function of position. 

\begin{table}
\begin{tabular}{c|c|c}
Variable & Estimate & Standard Error\\ \hline
 A [mrad * $l/V$] & -0.0072943 & 0.0000798469\\ \hline
 B [mrad / $V l$]& -0.04437 & 0.00105311\\ \hline
 C [mrad] & -0.0304106 &  0.00215033\\ \hline
$l_{\rm hyb}$ [$l$] & 0.322342 & 0.00682202\\ \hline
$\tau$ [1/V] & 0.200372 & 0.0110157
%%
%%{
%% {-0.0072943, 0.0000798469},
%% {-0.04437, 0.00105311},
%% {-0.0304106, 0.00215033},
%% {0.322342, 0.00682202},
%% {0.200372, 0.0110157}
%%}
\end{tabular}
\caption{Fit parameters of Eq. \eqref{eq:thetaFit}, where $l = \SI{5}{\micro\meter}$ is the length of the junction. Note that $\tau$ enters as $\mu \tau$ in $f(\mu)$. At the same time, $\mu = \text{const.} V_\mathrm{g}$, where empirically $\text{const.} \sim 1/200$ (i.e. 1 V of gate voltage changes the chemical potential by 5 meV). The presented value for $\tau$ does not accommodate for the empirical correction factor, but physically our best fit $1/\tau \sim \SI{5}{V}$ corresponds to a physical decay rate $1/\tau \sim \SI{25}{meV}$, which is realistic.}
\label{tab:TabValues}
\end{table} 
% \begin{figure}
% \includegraphics[width = .4\textwidth]{KerrExpAll.png}
% \includegraphics[width = .4\textwidth]{KerrExpAvg.png}
% \includegraphics[width = .4\textwidth]{KerrExpWOAvg.png}
% \includegraphics[width = .4\textwidth]{BestFitKerr.png}
% \caption{Comparison of (from left to right): 1. The experimental Kerr Data, 2. the spatial average over the latter, 3. the difference between the first and the second, 4. theoretical fit to the third (paramters are given in Fig.~\ref{tab:TabValues}.}
% \label{fig:KerrFit}
% \end{figure}

\begin{figure}
\includegraphics[scale=1]{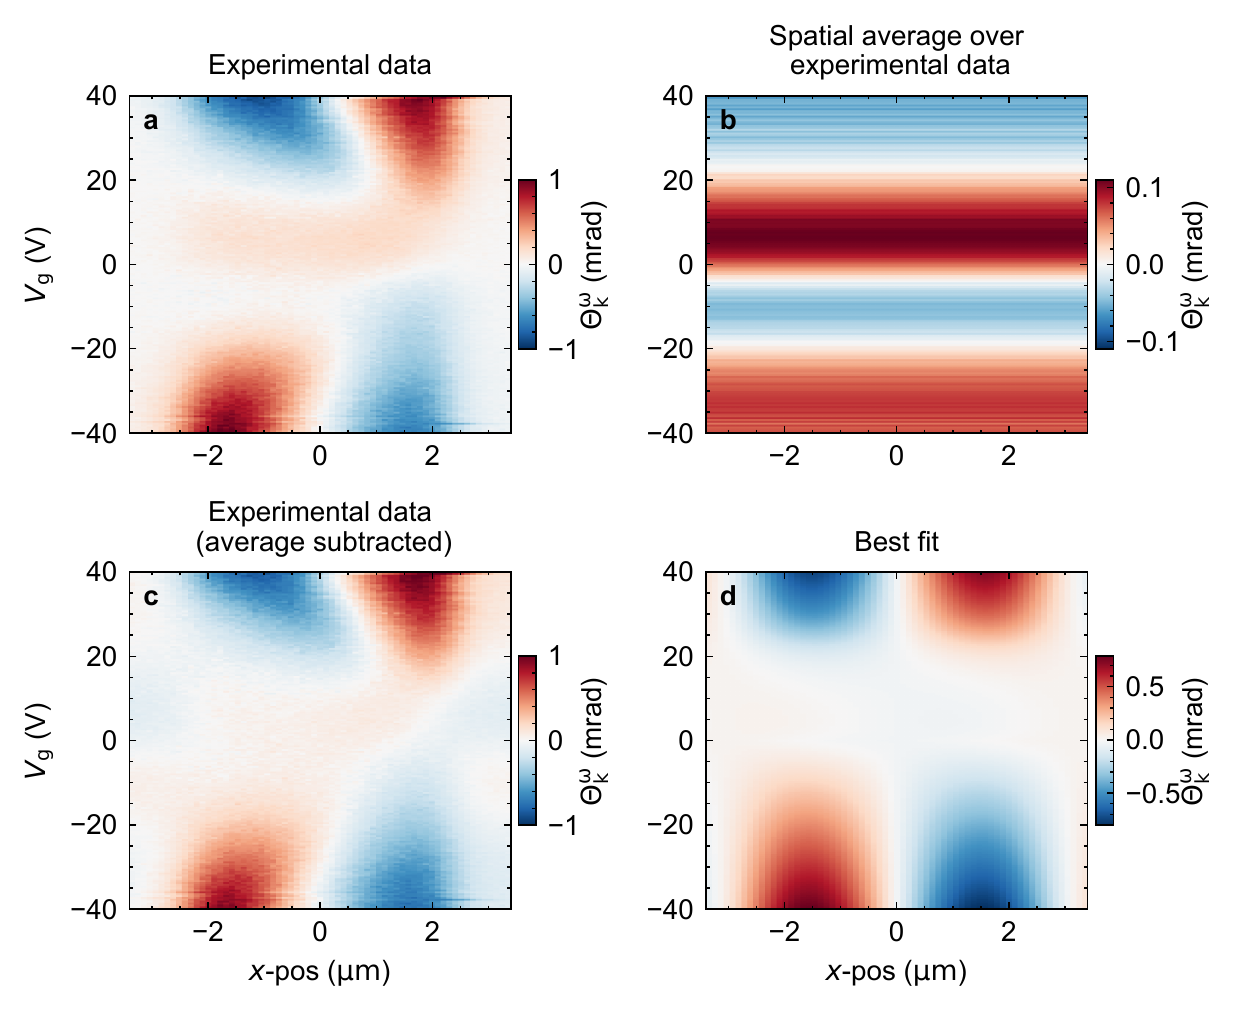}
\caption{\textbf{Theory of current-induced KR in \ch{WTe2}.} (a) The experimental Kerr Data, (b) the spatial average over the latter, (c) the difference between the \textit{(a)} and \textit{(b)}, (d) theoretical fit to \textit{(c)} (paramters are given in Tab.~\ref{tab:TabValues}). Panels (a) and (d) are also reported in Fig. 4 of the main text.}
\label{fig:KerrFit}
\end{figure}
